# Supplementary material for: Scattered Forest Search: Smarter Code Space Exploration with LLMs
Source: arXiv:2411.05010 source file (2025-02-25)
Supplement: Supplementary file 1 [file inference_scaling.tex]

\section{\revision{Trade-off between training and inference}}
\revision{
We provide a more detailed discussion of the tradeoff between training and inference here. 
}
