# Supplementary material for: Scattered Forest Search: Smarter Code Space Exploration with LLMs
Source: arXiv:2411.05010 source file (2025-02-25)
Supplement: Supplementary file 2 [file similarity.tex]

\begin{table}[ht]
    % \small
    \centering
    \caption{\textbf{Average similarity of different search methods.} }
    \begin{tabular}{c c c c c c c c}
    \toprule
    \multirow{2}{*}{\textbf{Benchmark}} & \multirow{2}{*}{\shortstack{\textbf{Ground truth}\\\textbf{tests given}}} & \multicolumn{6}{c}{\textbf{Pass@1 performance per method}} \\ \cmidrule(lr){3-8} 
    & & Random & Line & Tree & \scatter & \scout & Forest \\ \midrule
    \multirow{3}{*}{\textbf{HumanEval+}} & No tests given & & & & & & \\
    & 2 tests given & & & & & & \\
    & All tests given & & & & & & \\ \midrule
    \multirow{3}{*}{\textbf{MBPP+}} & No tests given & & & & & & \\
    & 1 test given & & & & & & \\
    & All tests given & & & & & & \\
    \bottomrule
    \end{tabular}
    \label{tab:correct_tests}
\end{table}
