# Supplementary material for: Scattered Forest Search: Smarter Code Space Exploration with LLMs
Source: arXiv:2411.05010 source file (2025-02-25)
Supplement: Supplementary file 3 [file test_generation.tex]

\section{\revision{Test generation}}
\revision{
Since problems and coding prompts do not usually come with unit tests, we need to generate unit tests ourselves 
}
